# Supplementary material for: Cataclysmic Variables from Sloan Digital Sky Survey V -- the search for period bouncers continues
Source: arXiv:2305.13371 source file (2023-09-11)
Supplement: Supplementary file 1 [file CVs_from_SDSS_V_plate_survey__1_Supplementary_information.pdf]

# Cataclysmic Variables from Sloan Digital Sky Survey V - the Plate Survey. Supplementary material

21 May 2023

## 1 INTRODUCTION

We include here all of the supplementary material supporting the main paper which could not be included because of its size.

## 2 SPECTRA AND LIGHT CURVES OF PREVIOUSLY KNOWN CVS

This paper has been typeset from a T<sub>E</sub>X/L<sup>A</sup>T<sub>E</sub>X file prepared by the author.

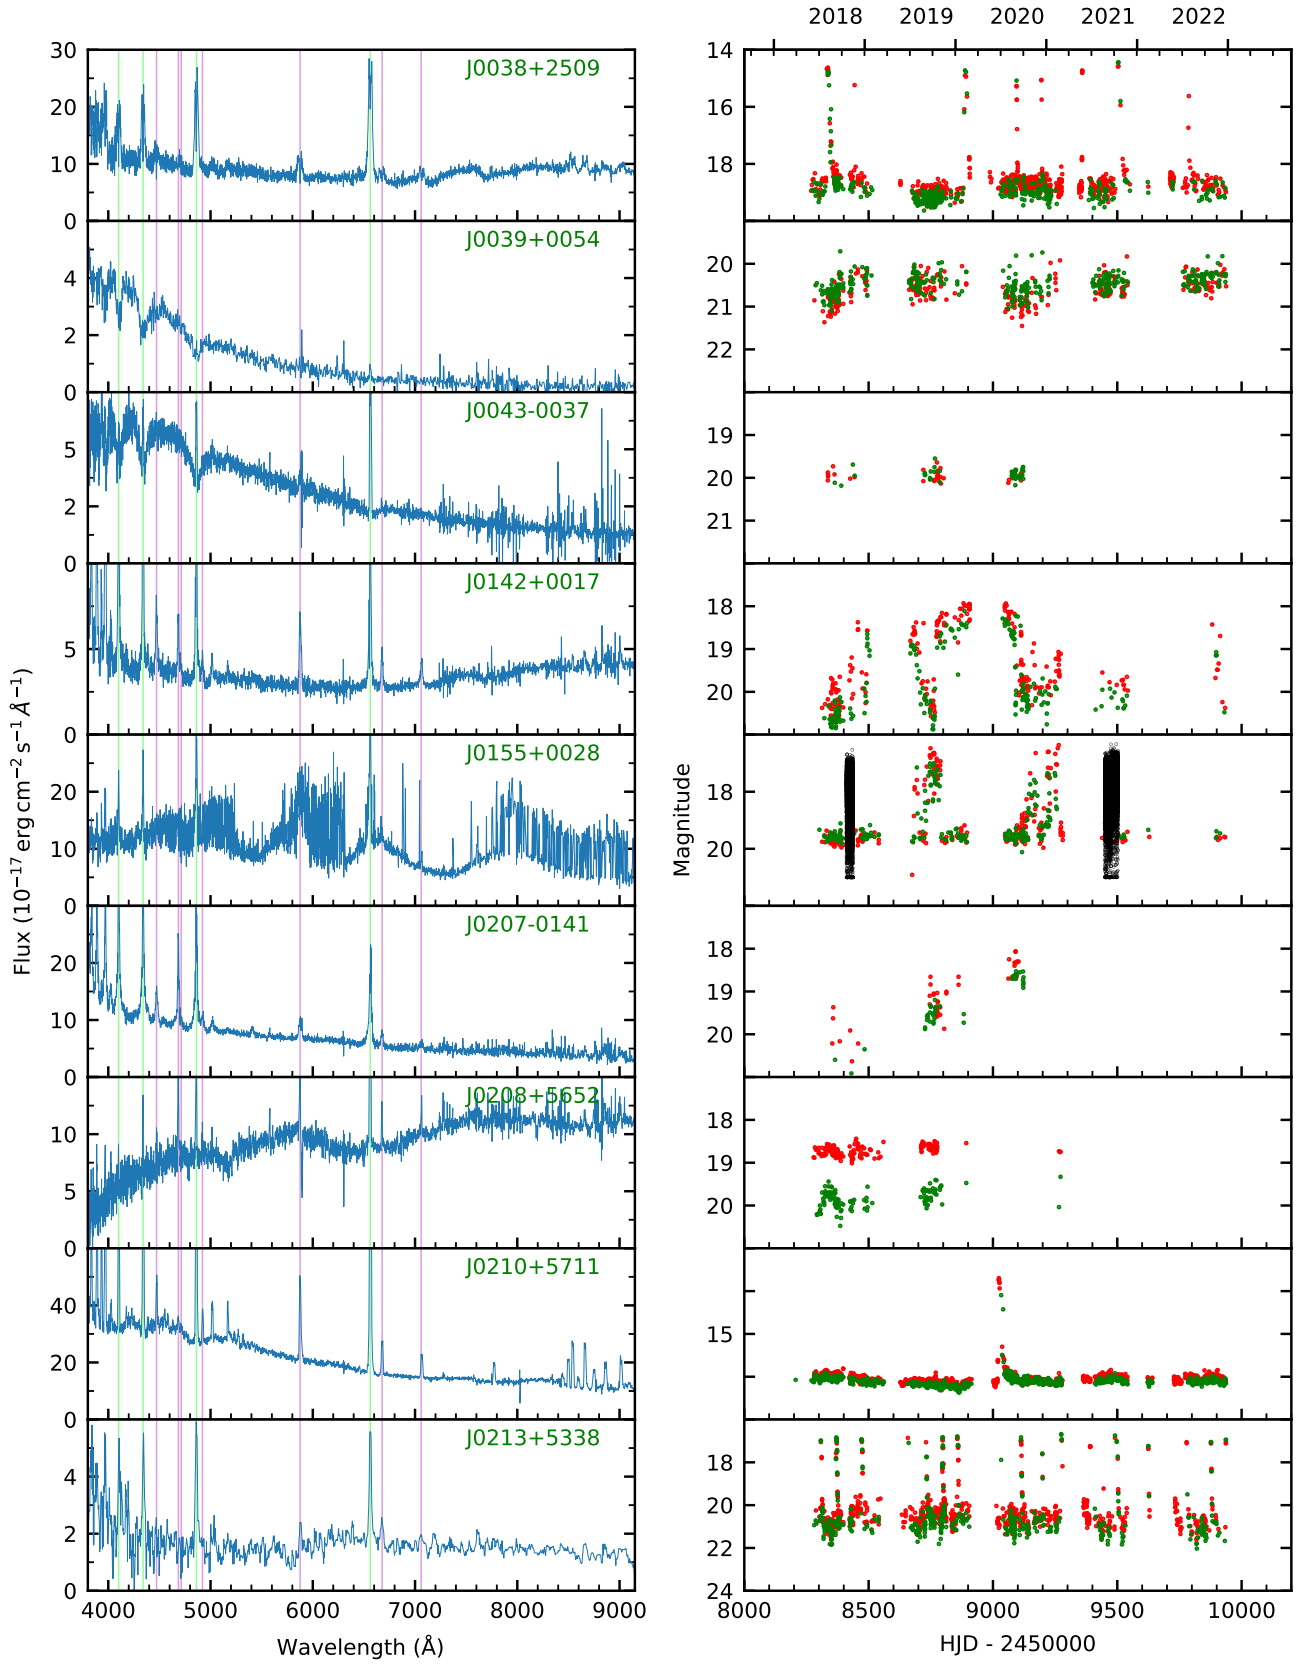

**Figure 1.** Left panels: Spectra of the CVs previously known by SDSS-V. Right panels: ZTF light curves of the previously known CVs (*r*- and *g*-band). TESS light curves are shown in black.

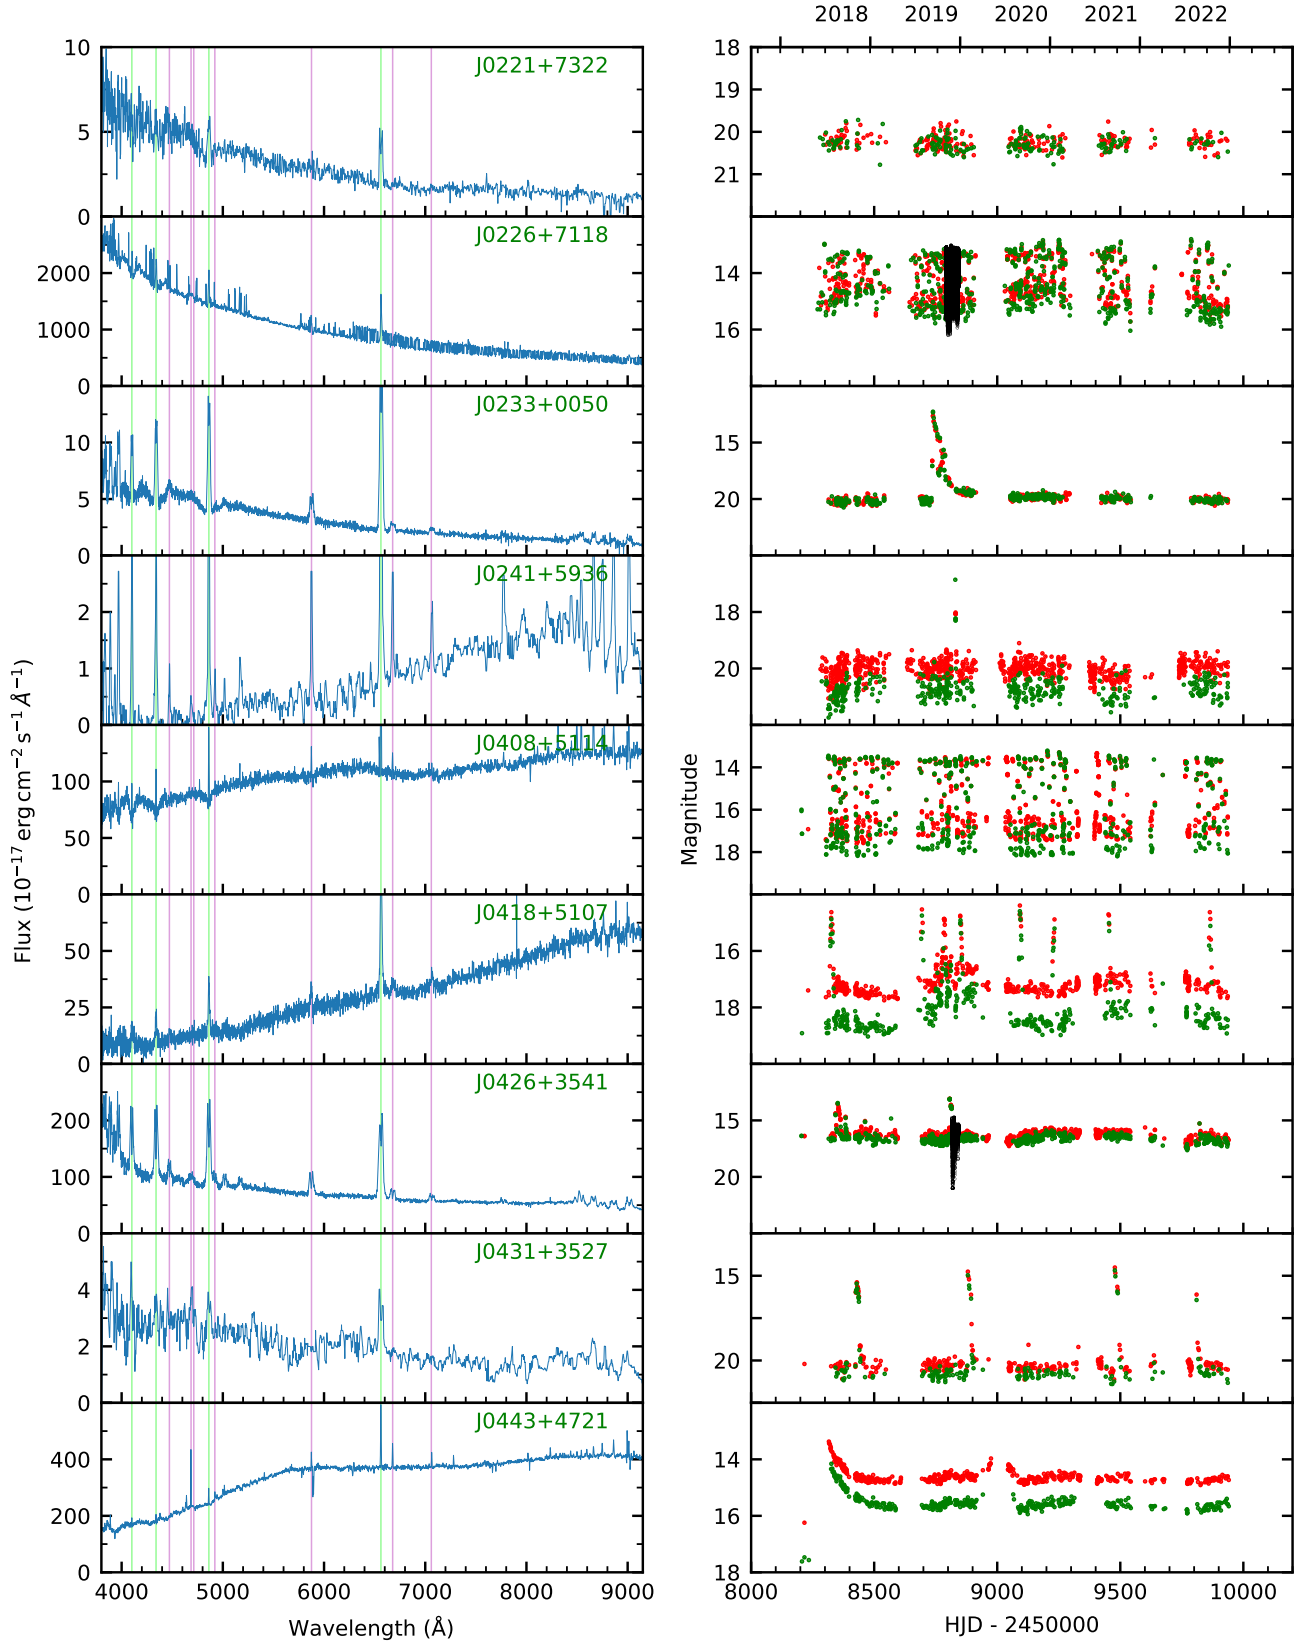

**Figure 2.** Left panels: Spectra of the CVs previously known by SDSS-V. Right panels: ZTF light curves of the previously known CVs ( $r$ - and  $g$ -band). TESS light curves are shown in black.

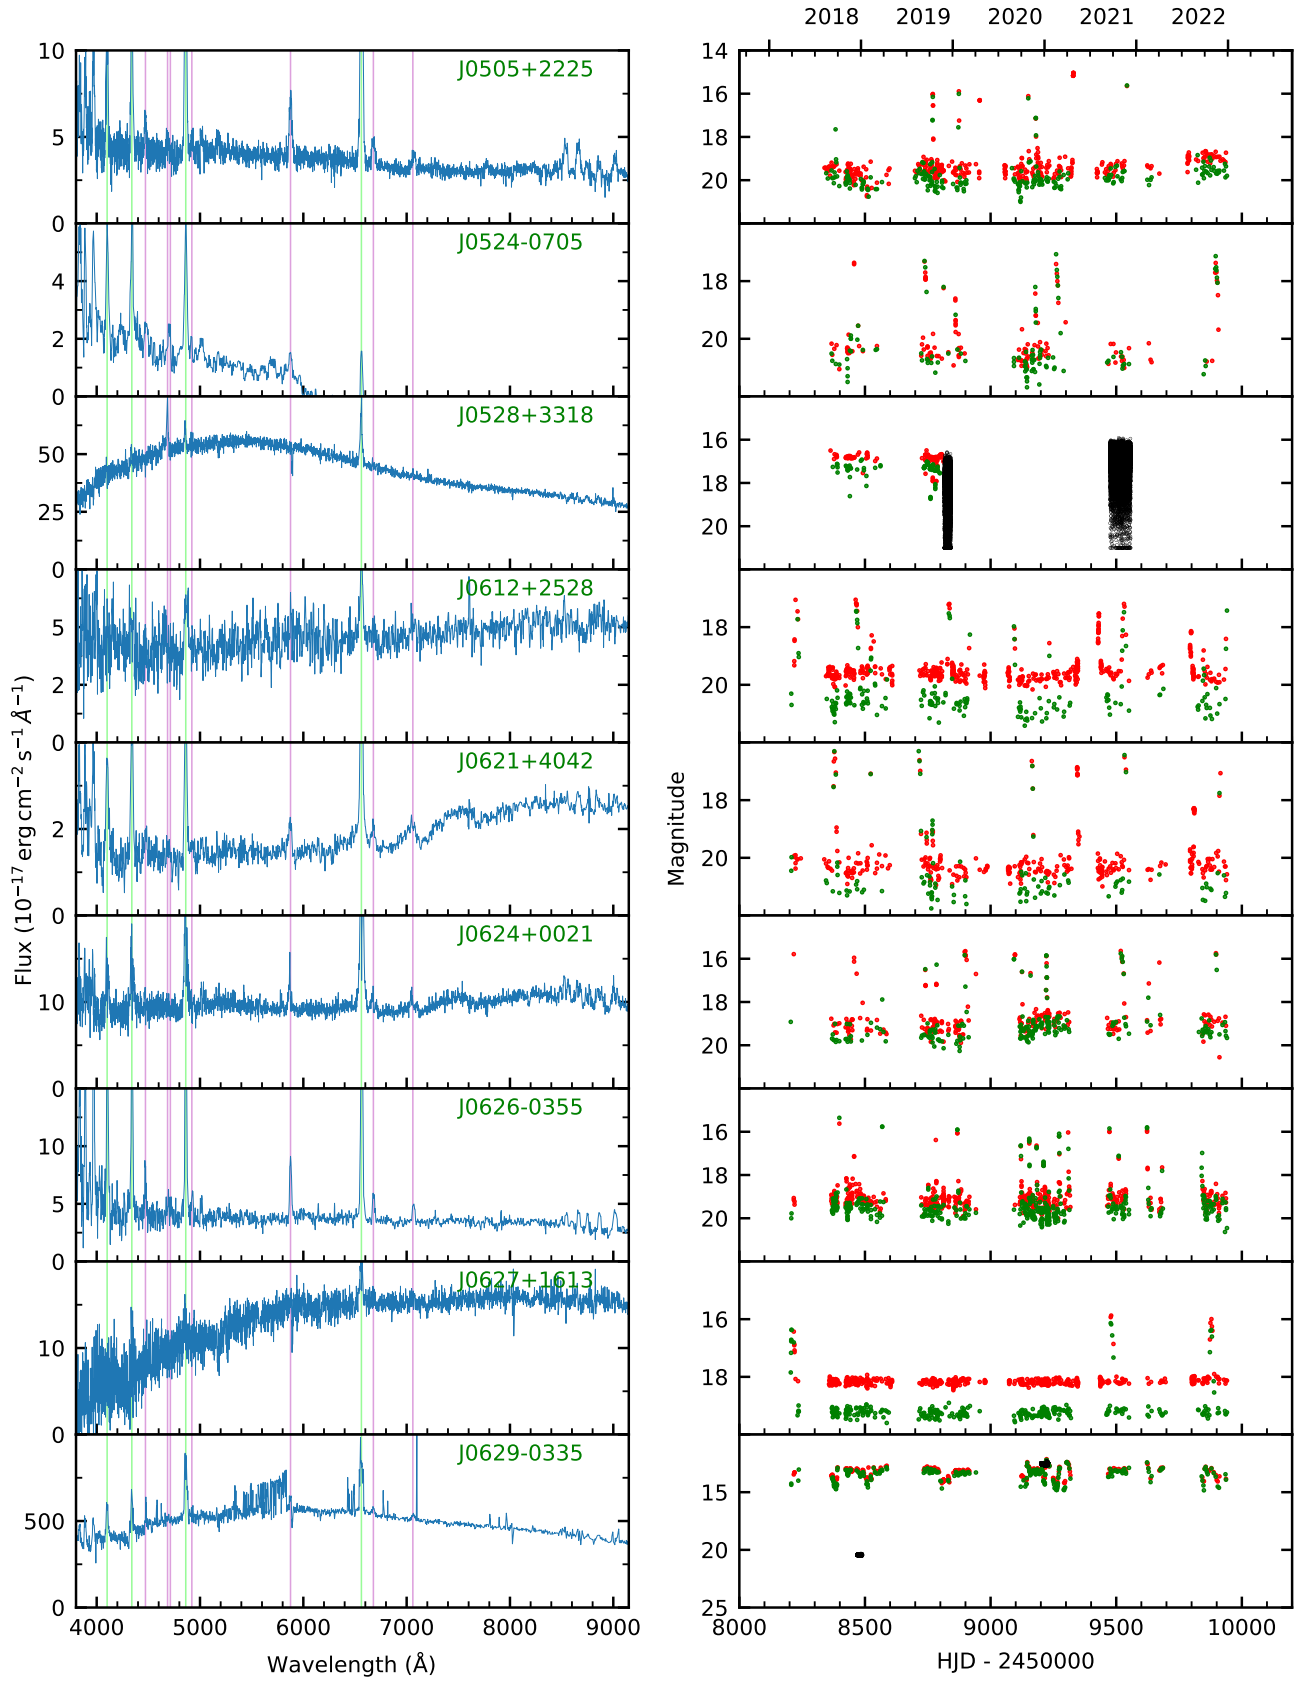

**Figure 3.** Left panels: Spectra of the CVs previously known by SDSS-V. Right panels: ZTF light curves of the previously known CVs (*r*- and *g*-band). TESS light curves are shown in black.

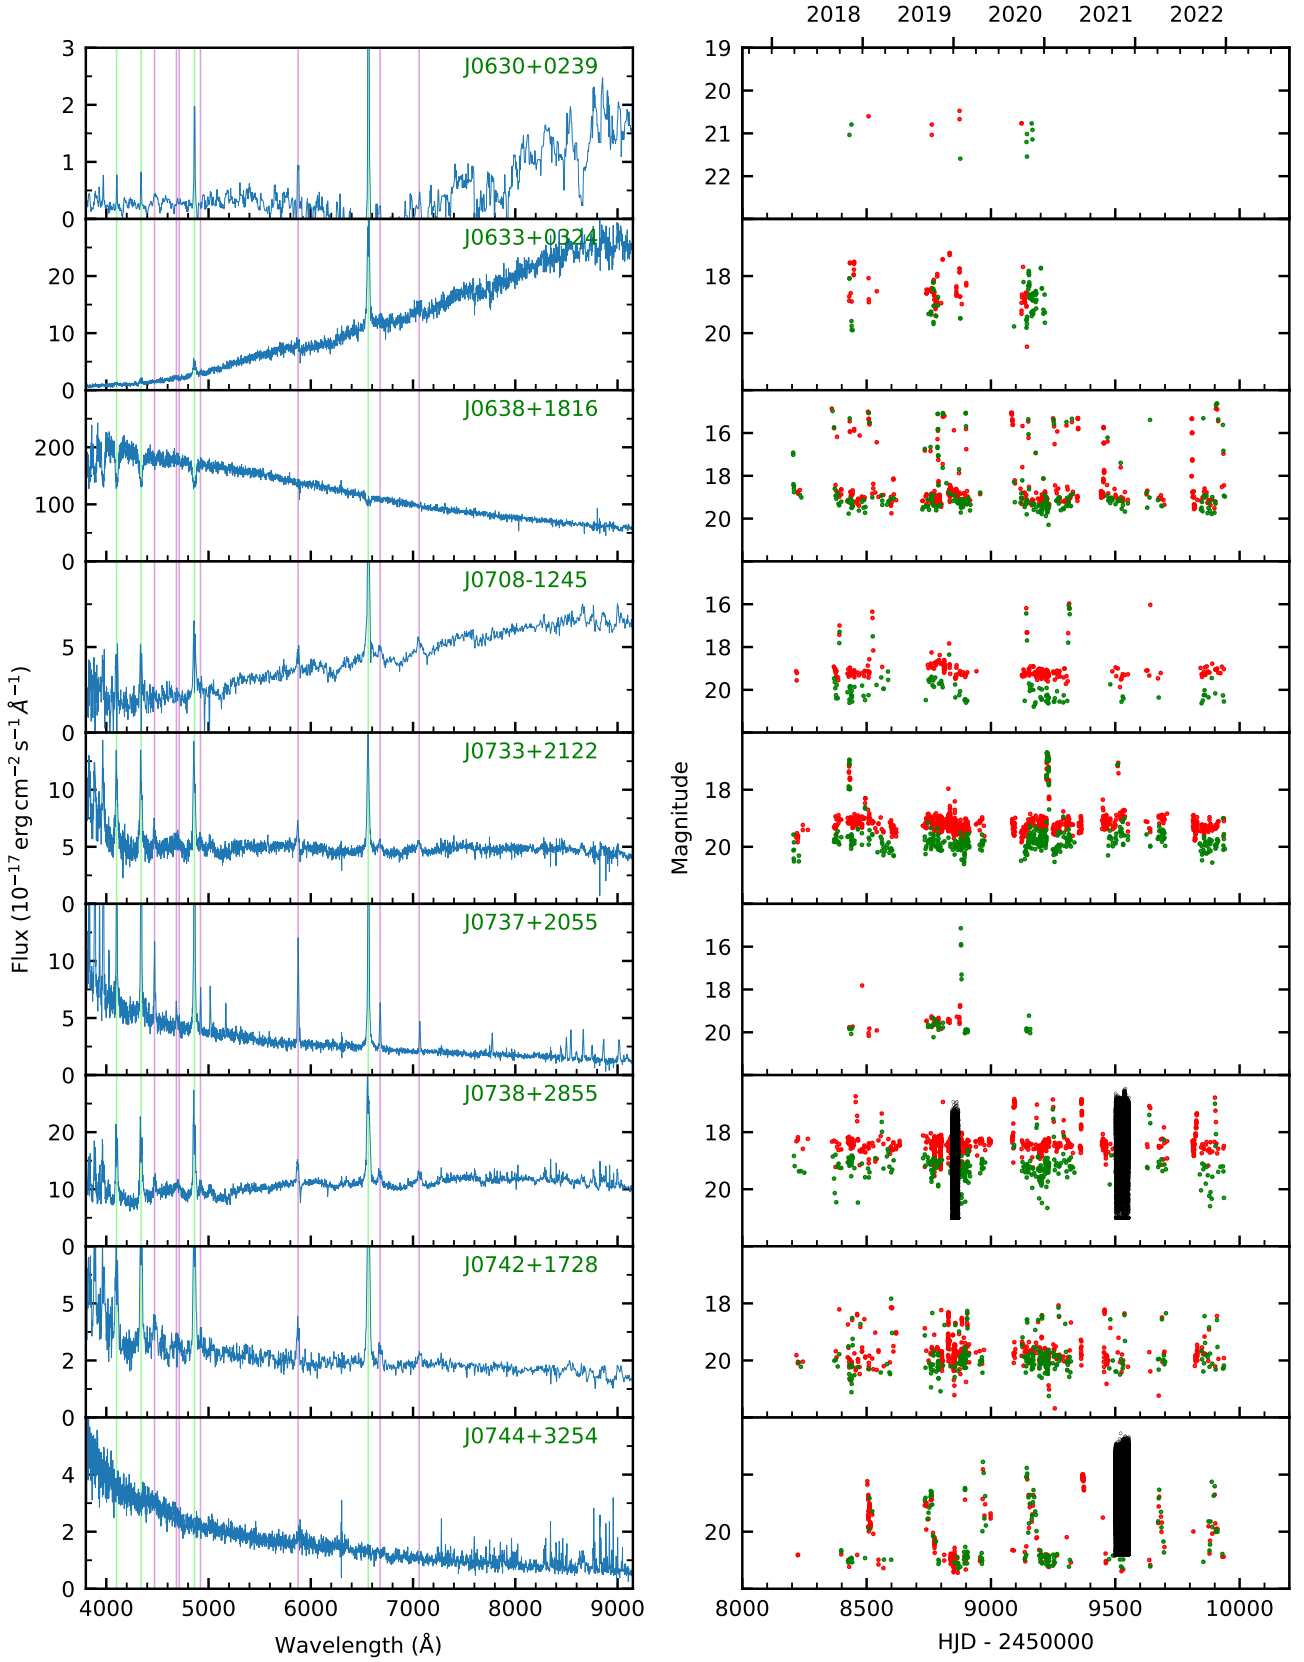

**Figure 4.** Left panels: Spectra of the CVs previously known by SDSS-V. Right panels: ZTF light curves of the previously known CVs (*r*- and *g*-band). TESS light curves are shown in black.

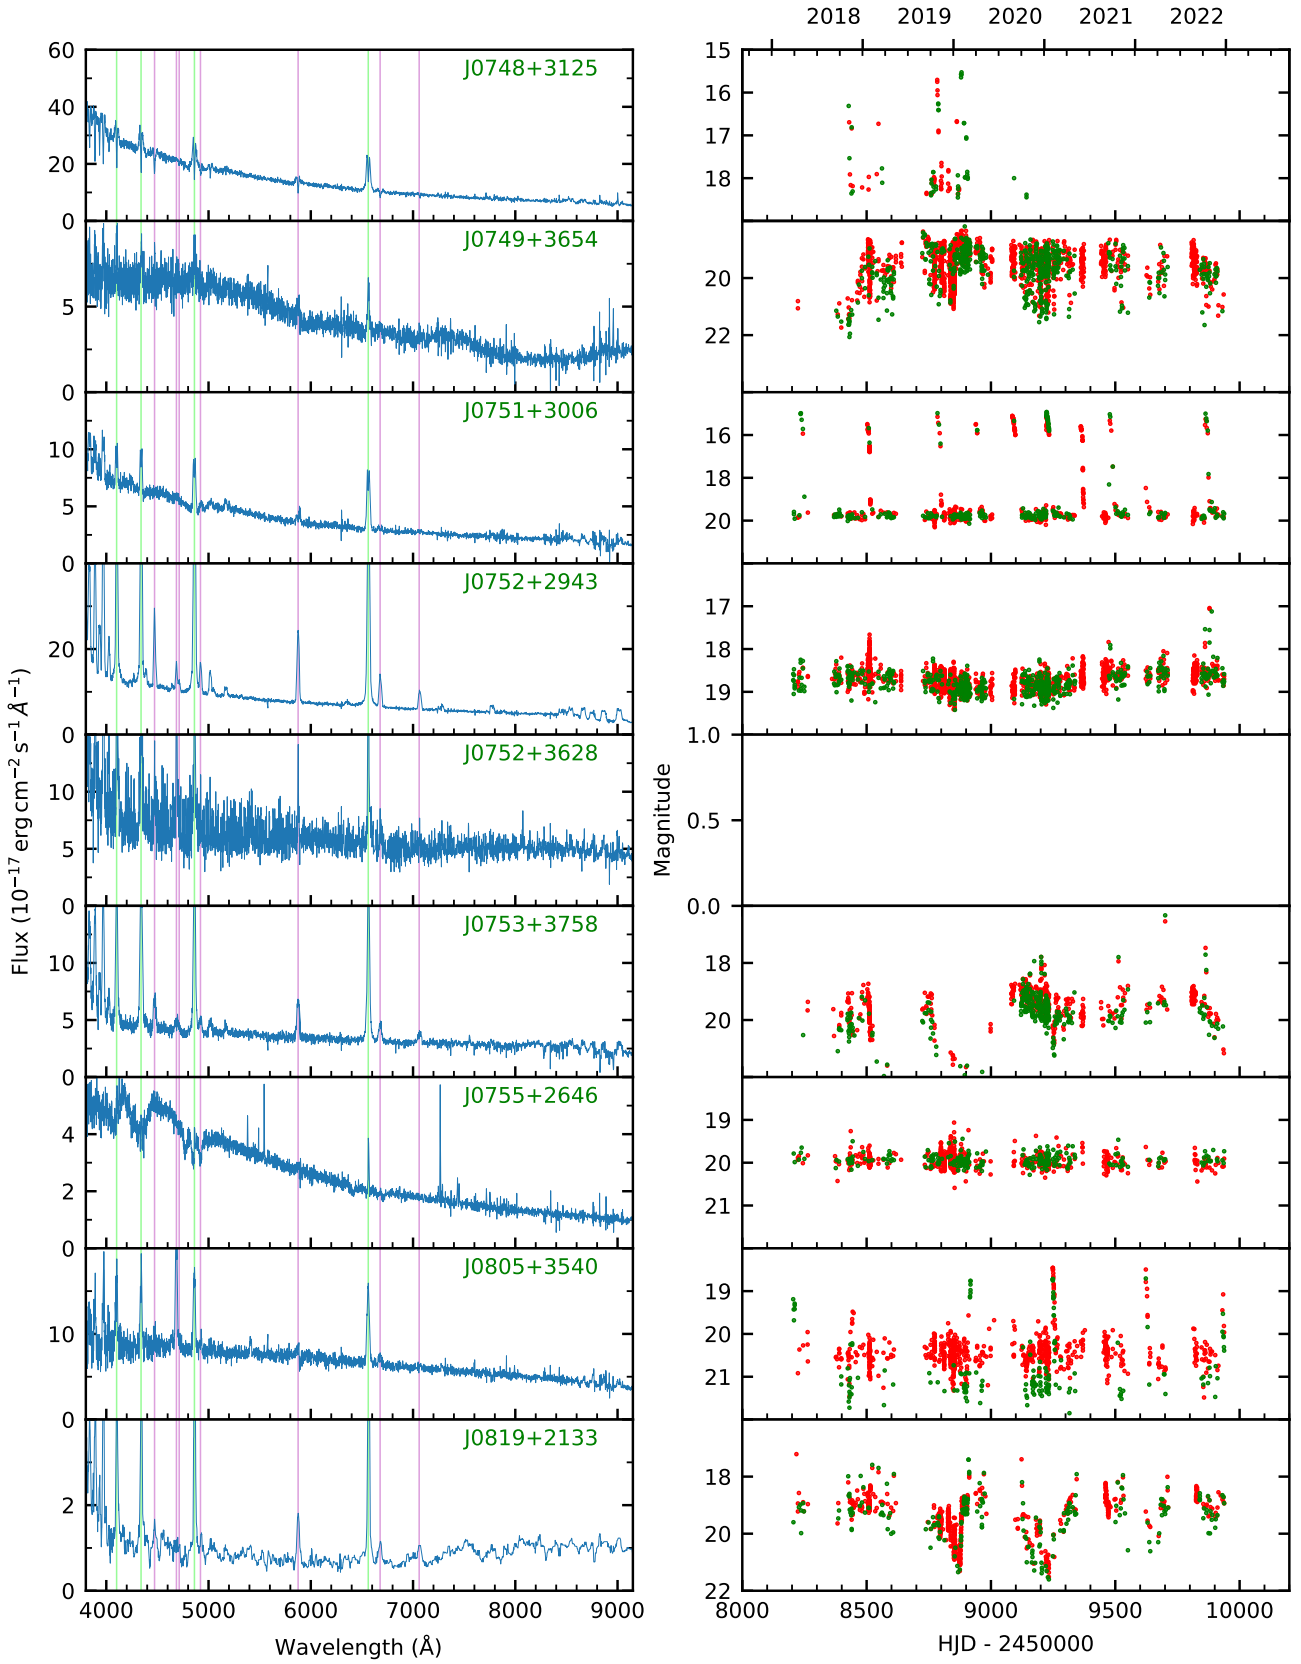

**Figure 5.** Left panels: Spectra of the CVs previously known by SDSS-V. Right panels: ZTF light curves of the previously known CVs (*r*- and *g*-band). TESS light curves are shown in black.

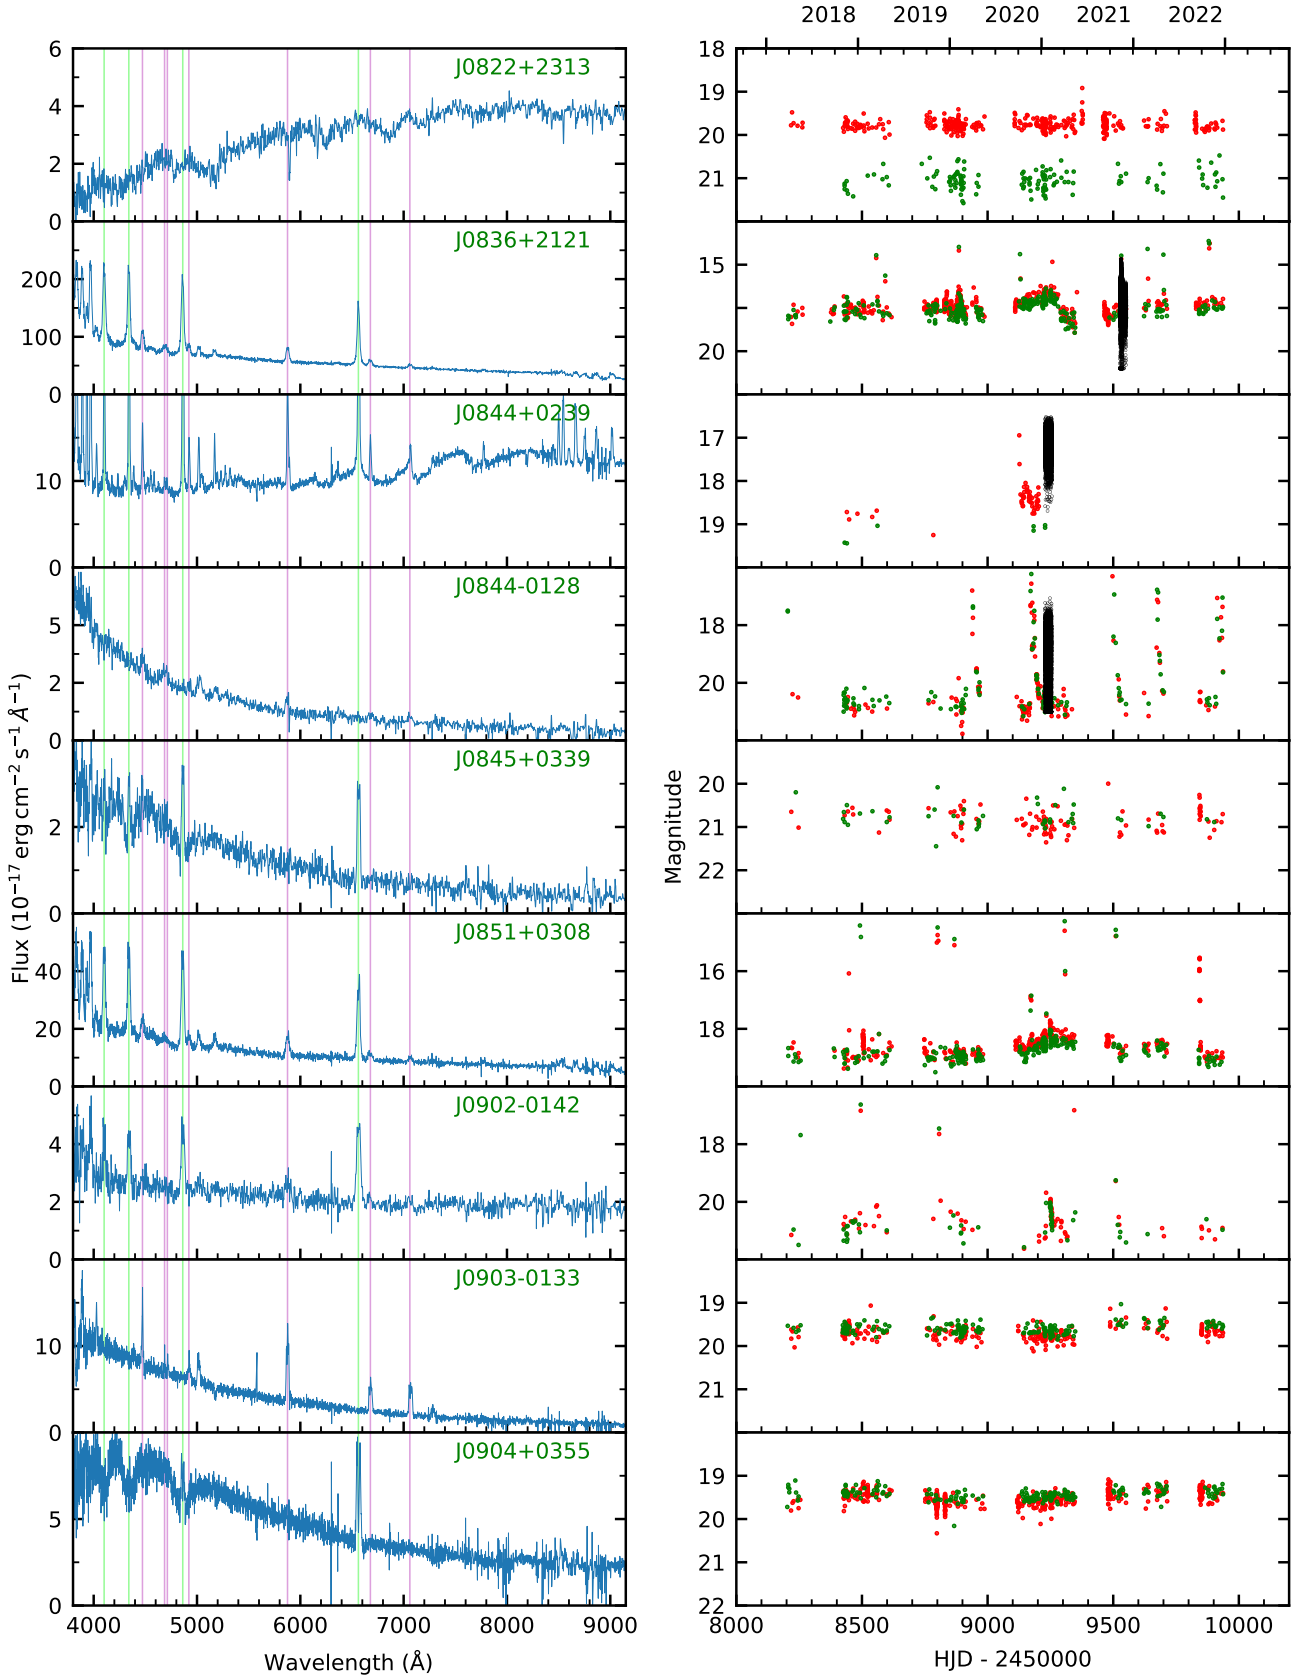

**Figure 6.** Left panels: Spectra of the CVs previously known by SDSS-V. Right panels: ZTF light curves of the previously known CVs (*r*- and *g*-band). TESS light curves are shown in black.

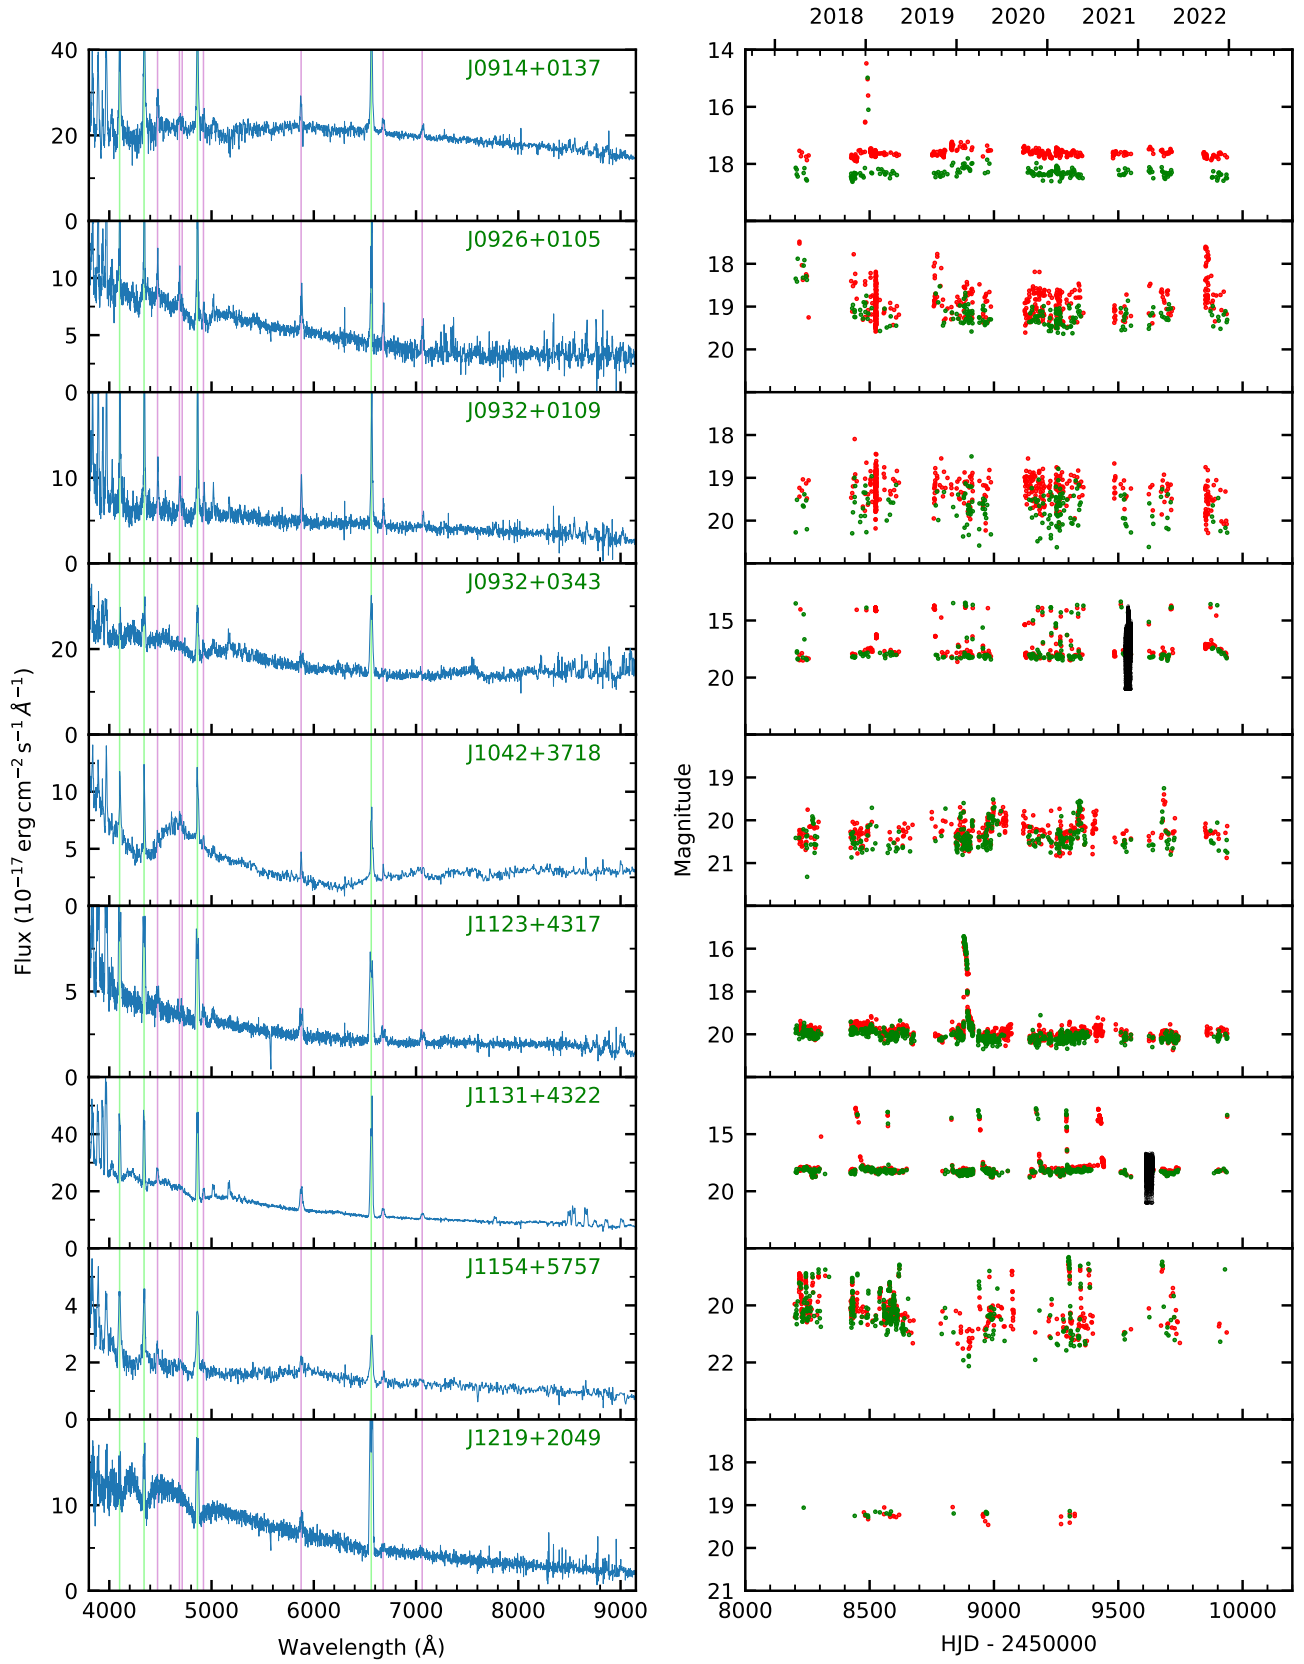

**Figure 7.** Left panels: Spectra of the CVs previously known by SDSS-V. Right panels: ZTF light curves of the previously known CVs (*r*- and *g*-band). TESS light curves are shown in black.

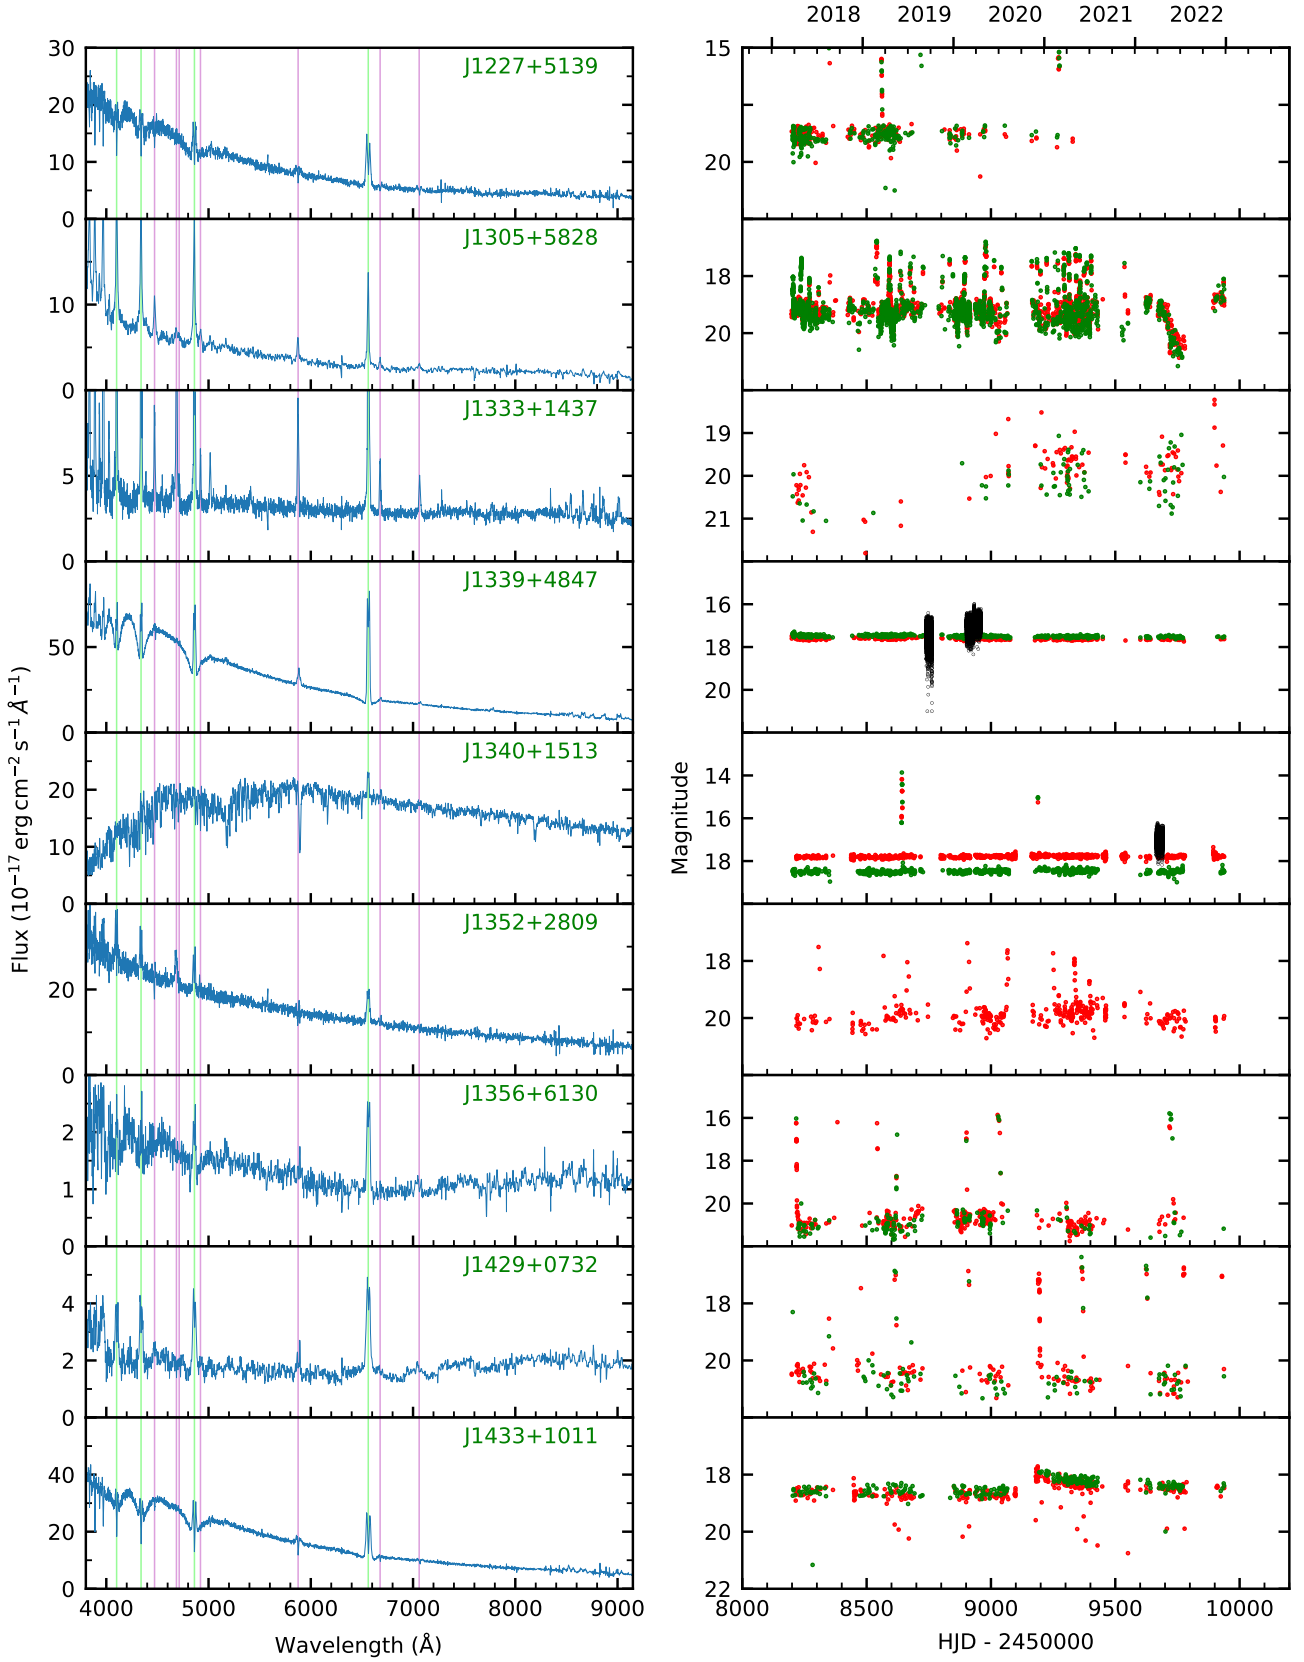

**Figure 8.** Left panels: Spectra of the CVs previously known by SDSS-V. Right panels: ZTF light curves of the previously known CVs (*r*- and *g*-band). TESS light curves are shown in black.

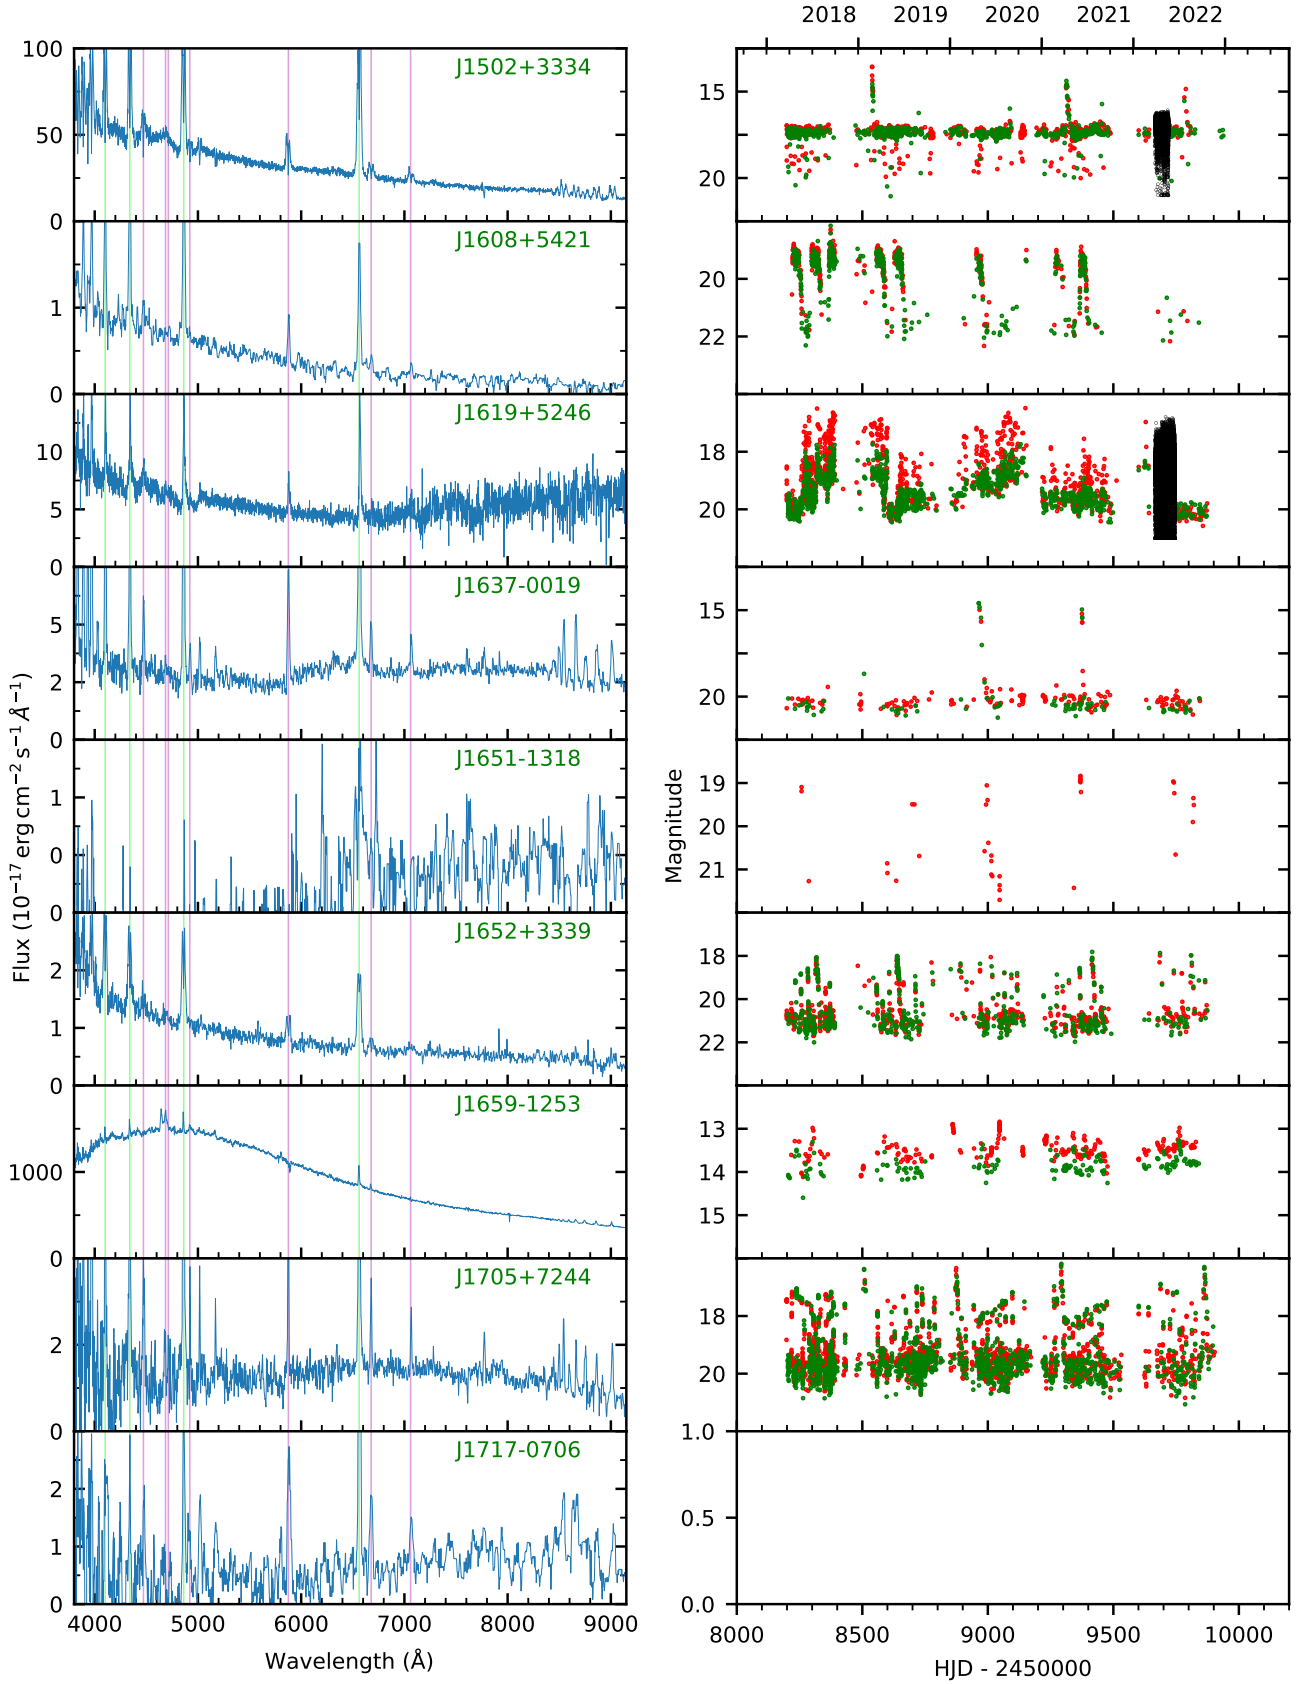

**Figure 9.** Left panels: Spectra of the CVs previously known by SDSS-V. Right panels: ZTF light curves of the previously known CVs (*r*- and *g*-band). TESS light curves are shown in black.

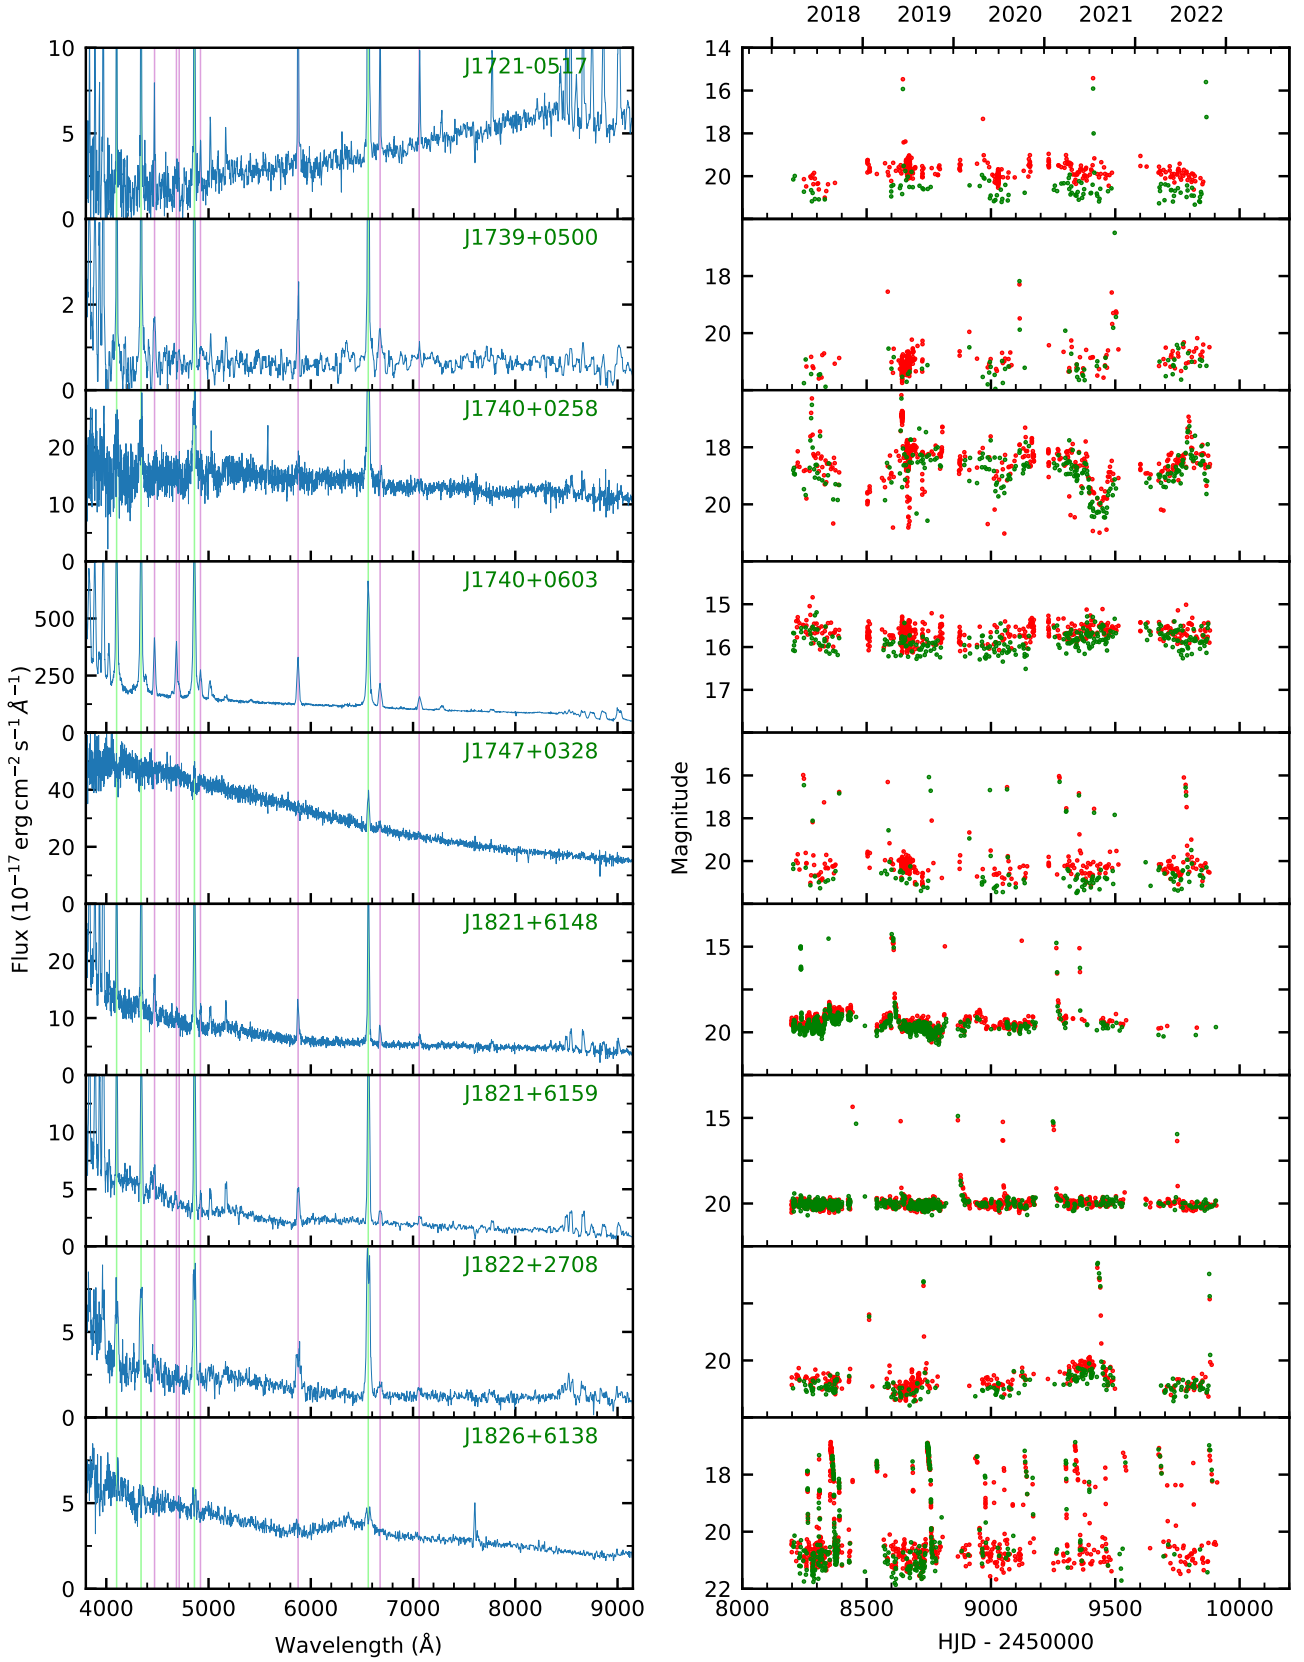

**Figure 10.** Left panels: Spectra of the CVs previously known by SDSS-V. Right panels: ZTF light curves of the previously known CVs (*r*- and *g*-band). TESS light curves are shown in black.

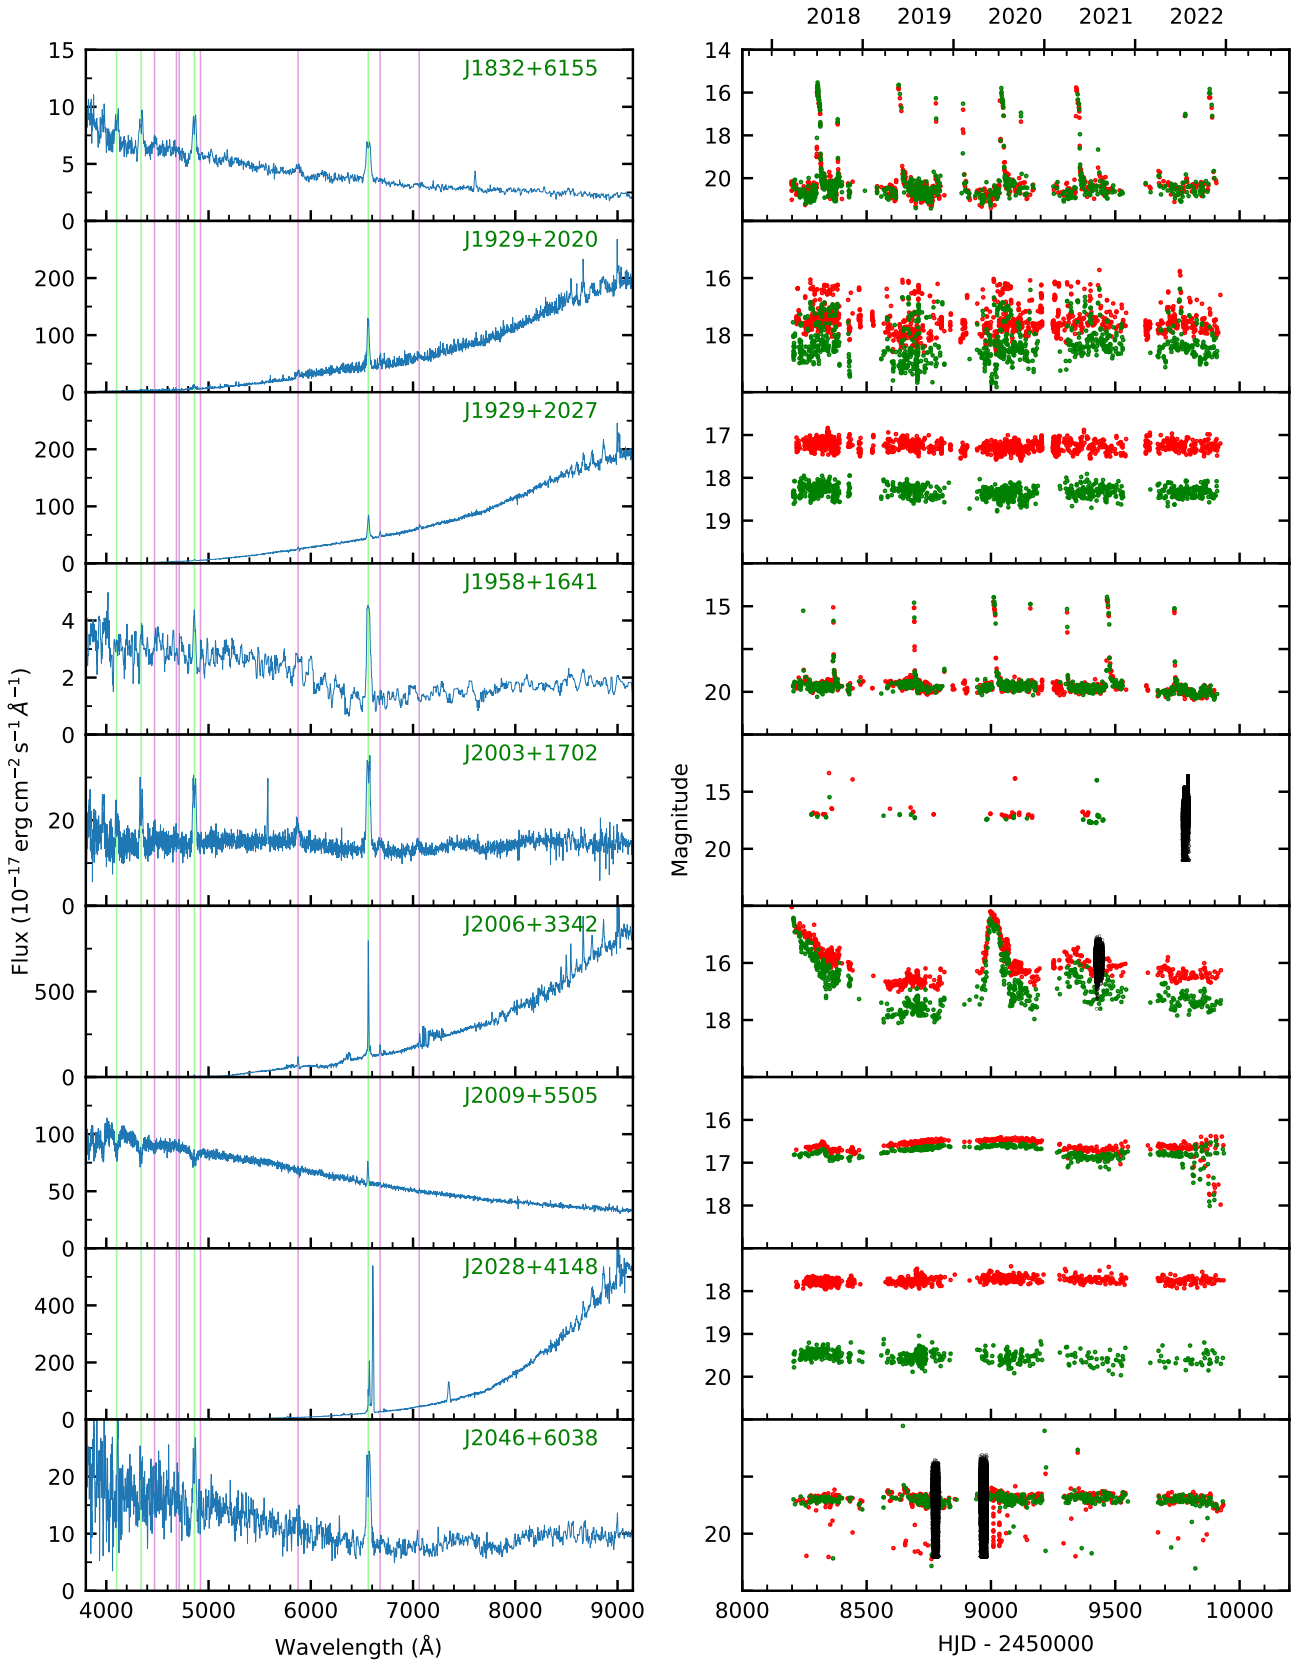

**Figure 11.** Left panels: Spectra of the CVs previously known by SDSS-V. Right panels: ZTF light curves of the previously known CVs (*r*- and *g*-band). TESS light curves are shown in black.

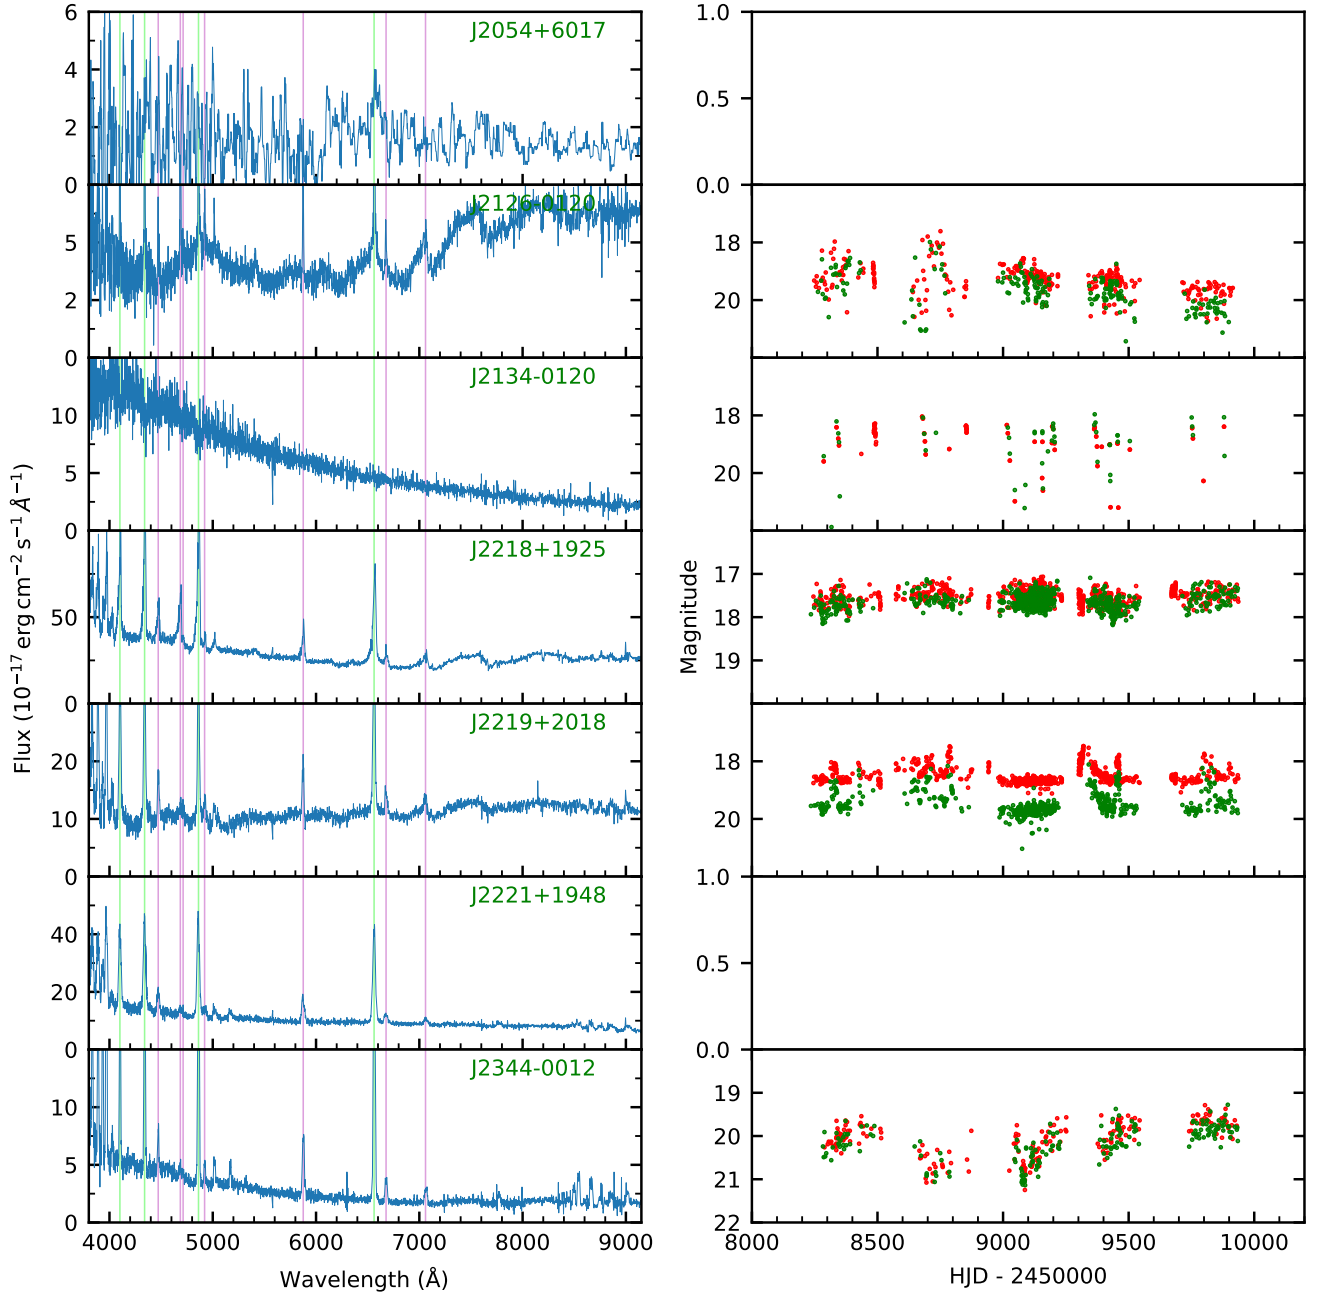

**Figure 12.** Left panels: Spectra of the CVs previously known by SDSS-V. Right panels: ZTF light curves of the previously known CVs (*r*- and *g*-band). TESS light curves are shown in black.

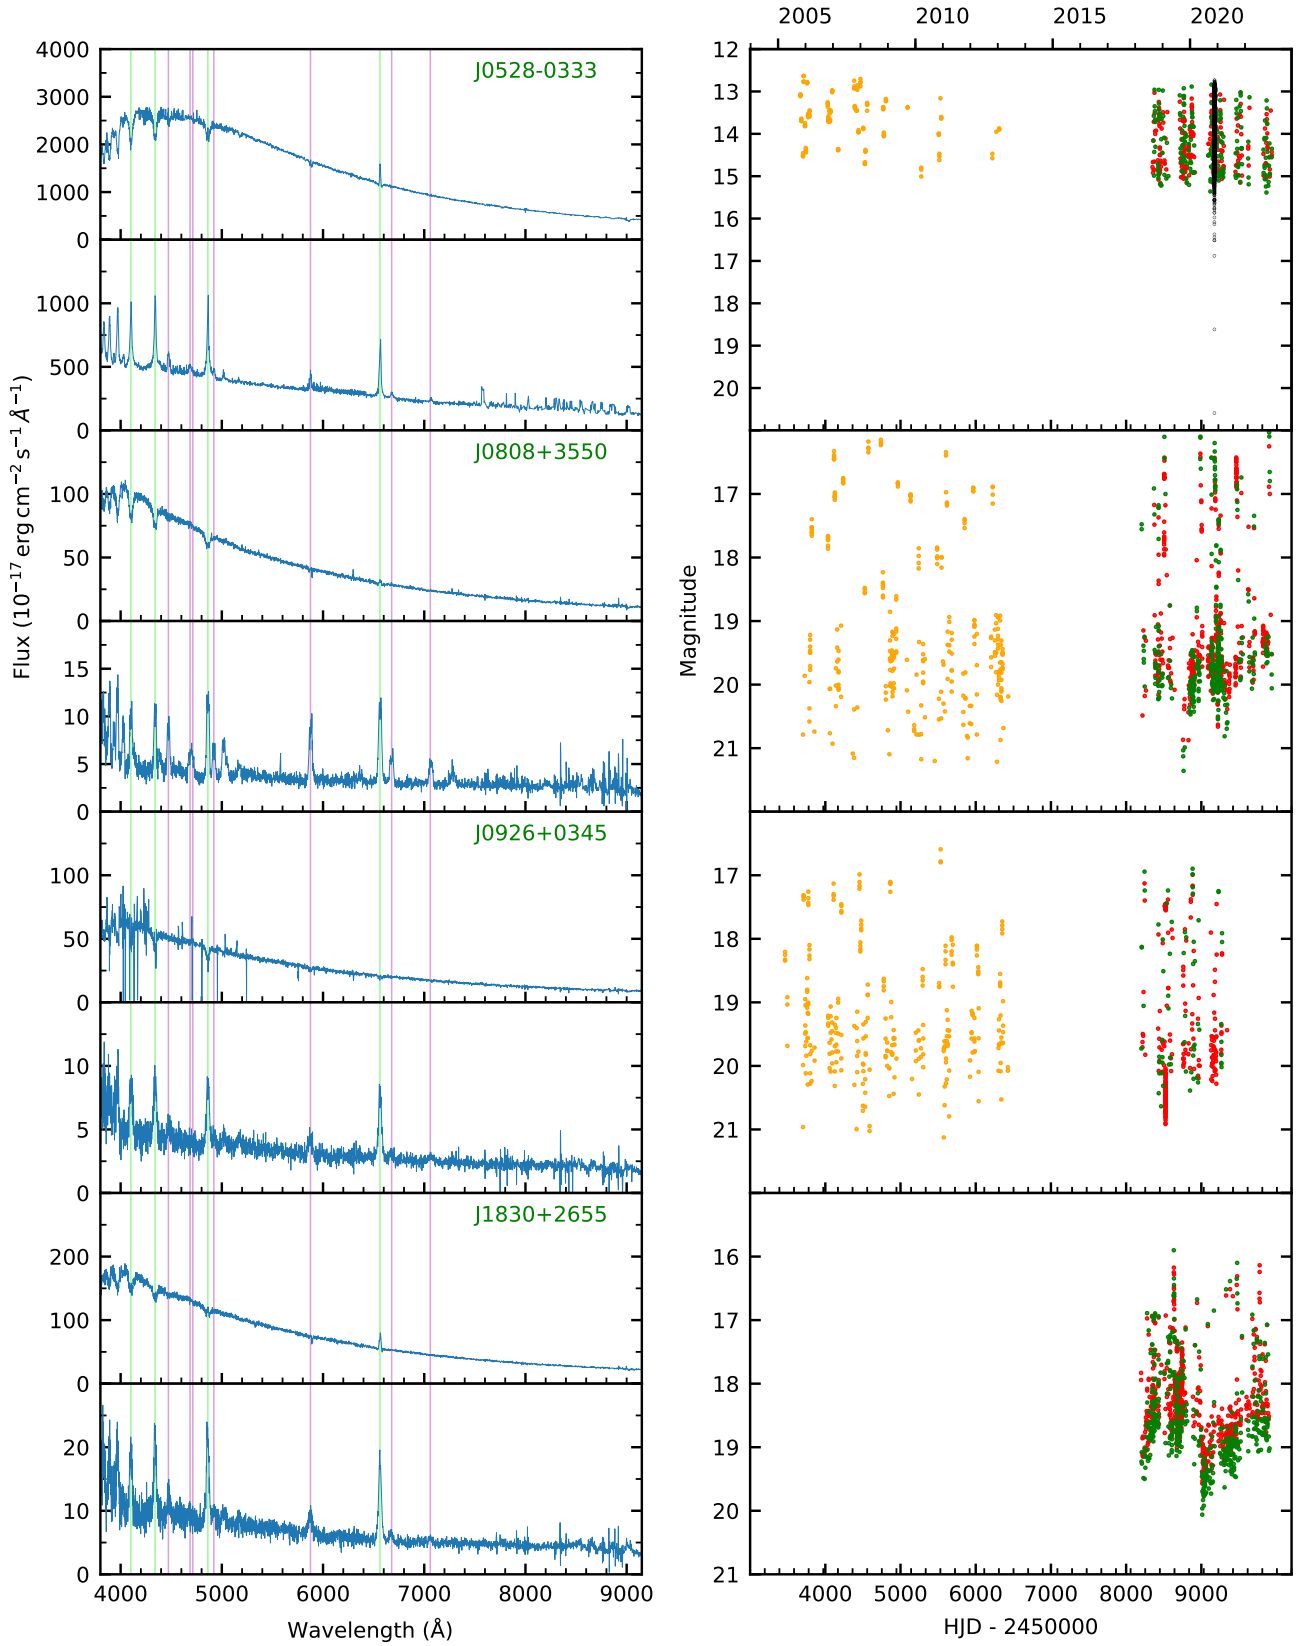

**Figure 13.** CV spectra in outburst (upper) and quiescence (lower). Left panels: Spectra of the CVs previously known by SDSS-V. Right panels: ZTF light curves of the previously known CVs (*r*- and *g*-band). TESS light curves are shown in black, CRTS in yellow.
